# Supplementary material for: What's Different between Visual Question Answering for Machine "Understanding" Versus for Accessibility?
Source: arXiv:2210.14966 source file (2022-10-26)
Supplement: Supplementary file 1 [file appendix.tex]

%\subsection{Implementation Details}\label{sec:implementation}
%We use three different code bases for our evaluation, which include OpenVQA (\url{https://github.com/MILVLG/openvqa}), Pythia (\url{https://github.com/allenai/pythia}), and ALBEF (\url{https://github.com/salesforce/ALBEF}).
%On the OpenVQA platform, four VQA models---MFB, BAN, BUTD, and MCAN---are already implemented. 
%Pythia supports both of the VQA-v2 and Vizwiz datasets, but the OpenVQA and ALBEF only support the VQA-v2 dataset. Thus, we implement the support of the VizWiz dataset on OpenVQA (i.e., for MFB, BAN, BUTD, and MCAN) and ALBEF.
%Their default hyperparameters are used to train models on VQA-v2 and VizWiz, respectively. For OpenVQA and ALBEF on which we implement the VizWiz support, the default hyperparameters for VQA-v2 are used to train models on VizWiz as well.
